# Supplementary material for: Accelerated Distributed Optimization with Compression and Error Feedback
Source: arXiv:2503.08427 source file (2025-03-29)
Supplement: Supplementary file 1 [file comparisons.tex]

\section{Comparisons of the Convergence Rates}
\label{sec:comparisons}

\begin{table*}[h]

    \caption{Comparison of key existing works on stochastic distributed optimization with contractive compression in the general convex regime.For simplicity, we assume that $L=\ell=L_{\max}$. We also assume the worst case scenario where the message compressed via $\cC$, $\delta$-contractive compression, transmit $\delta$ bits.
    }
    \label{tab:comparison-appendix}
    \centering
    \begin{tabular}{cccc}
        \toprule
        \textbf{Algorithm} & \textbf{Communication}  & \textbf{Oracle} & \textbf{Batch Size} \\
        \midrule
        \makecellnew{\algname{EF}\\\citep{seide20141}} & $\cO\left(\frac{\sqrt{L}R_0^2\zeta}{\varepsilon^{\nicefrac{3}{2}}} + \frac{LR_0^2}{\varepsilon}\right)$ & $\cO\left(\frac{R_0^2\zeta \sigma^2}{\sqrt{L}\varepsilon^{\nicefrac{5}{2}}} + \frac{R_0^2\sigma^2}{\delta\epsilon^2}\right)$ & $\cO\left(\frac{R_0^2\sigma^2}{n\varepsilon^2}+\frac{\sqrt{L}R_0^2(\nicefrac{\zeta}{\sqrt{\delta}}+\sigma)}{\sqrt{\delta}\varepsilon^{\nicefrac{3}{2}}}+\frac{LR_0^2}{\delta\varepsilon}\right)$\\
        \cmidrule{1-4}
        \makecellnew{\algname{EControl}\\\citep{gao2024econtrol}} & $\cO\left(\frac{LR_0^2}{\varepsilon}\right)$ & No & $\cO\left(\frac{R_0^2\sigma^2}{n\varepsilon^2}+\frac{\sqrt{L}R_0^2\sigma}{\delta^2\varepsilon^{\nicefrac{3}{2}}}+\frac{LR_0^2}{\delta\varepsilon}\right)$\\
        \cmidrule{1-4}
        \makecellnew{$\text{\algname{NEOLITHIC}}^{\rm (d)}$\\\citep{he2023lower}} & $\wtilde\cO\left(\frac{\sqrt{LR_0^2}}{\sqrt{\varepsilon}}\right)$ & Yes & $\wtilde\cO\left(\frac{R_0^2\sigma^2}{\delta n\varepsilon^2}+\frac{\sqrt{LR_0^2}}{\delta\sqrt{\varepsilon}}\right)^{\rm (e)}$\\
        \cmidrule{1-4}
        \makecellnew{\algname{\irick{Name?}}} & $\cO\left(\frac{\sqrt{LR_0^2}}{\delta\sqrt{\varepsilon}}\right)$ & No & $\cO\left(\frac{R_0^2\sigma^2}{n\varepsilon^2}+ \frac{\sqrt{L}R_0^2\sigma}{\delta^2\varepsilon^{\nicefrac{3}{2}}}+\frac{\sqrt{LR_0^2}}{\delta^2\sqrt{\varepsilon}} \right)$\\
        \bottomrule
    \end{tabular}
    \vspace{0.5em}
    \begin{tablenotes}
        {\scriptsize
        \item (b) BGS stands for Bounded Gradient Similarity assumption: $\avg{i}{n}\norm{\nabla f_i(\xx)-\nabla f(\xx)}^2\leq \zeta^2,\forall \xx\in\R^d$.
        \item (c) The rate is in terms of the number of communication rounds from the client to the server. We compare the rates when all algorithms take the same batch size between each updates.
        \item (d) \citet{he2023lower} presented their rates when batch size is $\max\{\frac{4}{\delta}\ln(\frac{4}{\delta}), \frac{1}{\delta}\ln(24\kappa + \frac{25n^2\kappa^3\zeta^4}{\sigma^4}+5n\kappa^{\nicefrac{3}{2}})\}$ where $\kappa$ is the total number of updates at the server. We present the rates when the batch size is one for a fair comparison. We also note that, in the worst case, \algname{NEOLITHIC} transmit more bits than simply sending the uncompressed vector between each update at the server and is therefore an uncompressed method.
        \item (e) $\wtilde\cO$ hides logarithmic factors in $\nicefrac{1}{\varepsilon}$.
        }
    \end{tablenotes}
\end{table*}

In this section we further discuss the comparison of the convergence rate for differenct methods. Here we consider 2 criterions:
\begin{itemize}
    \item The number of bits communicated from the client to the server, where for simplicity we assume that a full vector takes 1 bit. In the worst case, the message compressed via $\cC$, $\delta$-contractive compression, transmit $\delta$ bits.
    \item The number of oracle calls to the stochastic gradient oracles by the local clients. Here we allow the algorithm to take any batch size to achieve the lowest communication cost in terms of the number of bits communicated from the client to the server, and we list the resulting local oracle complexity.
\end{itemize}

We note that while we in this section we allow the algorithms to take any batch sizes (which are in fact dependent on the target error $\varepsilon$, sometimes referred as mega-batch), we still point out that in many practical scenarios, smaller batch sizes are preferred over mega-batches, as they might lead to better generalization performance~\cite{wilson003general,lecun2012efficient,  keskar2017largebatch}. Furthermore, in many practical settings, mega-batches are unavailable or intractable to sample, e.g., in medical tasks~\cite{rieke2020future}; federated Reinforcement Learning~\cite{khodadadian2022federated, jin2022federated}; and multi-agent Reinforcement Learning~\cite{doan2019finite}. 

We summarize the results in
